# Supplementary material for: Information Design for Hybrid Work under Infectious Disease Transmission Risk
Source: arXiv:2312.04073 source file (2023-12-07)
Supplement: Supplementary file 1 [file MSOM-si.tex]

\documentclass[12pt]{article}

\title{Using the xr package on Overleaf}
\usepackage{xr}
\makeatletter

\newcommand*{\addFileDependency}[1]{% argument=file name and extension
\typeout{(#1)}% latexmk will find this if $recorder=0
% however, in that case, it will ignore #1 if it is a .aux or 
% .pdf file etc and it exists! If it doesn't exist, it will appear 
% in the list of dependents regardless)
%
% Write the following if you want it to appear in \listfiles 
% --- although not really necessary and latexmk doesn't use this
%
\@addtofilelist{#1}
%
% latexmk will find this message if #1 doesn't exist (yet)
\IfFileExists{#1}{}{\typeout{No file #1.}}
}\makeatother
\newcommand*{\myexternaldocument}[1]{%
\externaldocument{#1}%
\addFileDependency{#1.tex}%
\addFileDependency{#1.aux}%
}
\myexternaldocument{./MSOM_Submission/MSOM-main}

\begin{document}

In the file \texttt{MSOM-main.tex}, the introduction is section \ref{sec:approximation}.

\end{document}
