# Supplementary material for: Information Design for Hybrid Work under Infectious Disease Transmission Risk
Source: arXiv:2312.04073 source file (2023-12-07)
Supplement: Supplementary file 2 [file 6_-_Appendix.tex]

%!TEX root = Opt_Info_Provision_Hybrid.tex

%\newpage
\section{Appendix}
\subsection{Extension to infinite $\K$}
\noindent Observe that initially we assume that $\K$ is finite, however we can naturally more generally extend to distributional notions of agent's private benefit from work where $\K$ becomes uncountable. Namely, we suppose that instead that the agents' benefit from in-person work $v$ is now generated randomly according to an arbitrary distribution $G$ taking support on the positive reals. Observe that when $\K$ was finite this corresponded to any discrete distribution.

\noindent Suppose that instead amongst the continuum of agents. Observe that the in-person mass can instead be computed via $m(\theta) = \inf\{0 \leq u \leq 1: G^{-1}(u) \geq c_1(1-u)\theta+c_2(1-u)\}$ as again the equilibrium in-person mass will equilibriate between the in-person costs and the remote costs. This statement directly follows from Lemmas \ref{lemma:rectangular_curve} and \ref{lemma:compute_inperson_mass}. 

\noindent Observe that defining objective sets in $\R^\K$ becomes intractable as $\K$ becomes uncountable, however the reduction shown only depends on the intersections with these sets and the curve $\curve$ which can be parameterized by the in-person mass. Consequently, we lose nothing by instead defining the goal sets to be intervals of in-person mass which the platform finds acceptable for the initial mass allocation $\init$.



\subsection{Extending stateful capacity setting under continuous distributions $\dist$}
We generalize the linear program obtained in Proposition \ref{prop:stateful} to hold for more general continuous distributions $\dist$ over $\Theta = [0,M]$. 

\noindent Suppose instead that $\dist$ is some continuous distribution over $\Theta$ and assume that the increasing function expressing the \textit{minimal remote work capacity} $b(\cdot)$ is $\eta_1$-Lipschitz. Then the following proposition claims that we can obtain an $\epsilon$-approximation to the true optimal mechanism. 

\subsection{Extension to general stateful settings}
\noindent Suppose agents are initialized with position $\init$ and that the
Consider instead that we we consider an arbitrary collection of objective sets $\goal(\nu)$. Notice that as before we can without loss of generality consider that each objective set $\goal(\nu)$ is a union of a finite number of disjoint intervals contained in $[0,1]$ corresponding to the desired in-person mass.

\subsection{Approximating DeVericourt et al. \cite{de_vericourt_informing_2021}}
We provide a brief numerical study highlighting the comparison between the results we obtain using our framework and that presented in DeVericourt et al (\cite{de_vericourt_informing_2021}). 


\subsection{Proof of Lemma \ref{lemma:intervals}}
The proof is quite immediate since notice that $\curve = \cup_{i=1}^{\K}  \{z(\init,u): s_{k-1} \leq u \leq s_k\}$. Consequently, $\goal \cap \curve = \cup_{i=1}^{\K}  \big(\goal \cap \{z(\init,u): s_{k-1} \leq u \leq s_k\}\big)$.
However, notice $\{z(\init,u): s_{k-1} \leq u \leq s_k\}$ is a line segment in $\R^\K$ so its intersection with a convex, compact set $\goal \subset \R^\K$ is just another line segment $\{z(\init,u): \tilde{\omega}_k^1  \leq u \leq \tilde{\omega}_k^2\}$ for some constants $\tilde{\omega}_k^1, \tilde{\omega}_k^2$. Eliminating empty intervals and condensing the intervals if $\tilde{\omega}_{j}^2 = \tilde{\omega}_{j+1}^1$ for any $j$ yields the result.

\subsection{Proof of Lemma \ref{lemma:num_signals_bdd}}
The proof follows directly from Lemma 1 in \cite{candogan_optimality_2019}.


\subsection{Partial Adherence - \srs{Move to appendix or footnote}}
Consider instead that only a fraction $\gamma$ of the population is capable of being influenced by the planner and the remaining $1-\gamma$ agents behave is some heterogeneous fashion. This could be due to a different perceived cost function or agents that do not consider the platform for information. Under this setting, we can easily extend to cases where the remaining agents can also be influenced by external information sources so long as all agents and the planner commonly agree on a deterministic relationship between the behavior of the remaining $1-\gamma$ agents as a function of the posterior mean that is generated. This can be justified if over several iterations, agents who do consider the platform learn a relationship between the other $1-\gamma$ agents' behavior with relation to the posterior mean generated. Under this case, $\tilde{m}(\theta_i)$ which now takes the form:
\begin{align*}
    \tilde{m}(\param_i) &\coloneqq \inf\{0 \leq u \leq \gamma: G^{-1}(u+n(\theta_i)) \geq c_1(u+n(\theta_i))\theta_i+c_2(u+n(\theta_i)) \\
        &= max\{0, m(\param_i)\}
\end{align*}
Partial adherence models have been studied in further detail in Tavafoghi et al, Savla et al. \srs{Just come back to fill details on this later - it's not significant as is. Look at Manxi's paper for inspiration if struct can be adapted. As is this is not general since under multiple information systems, I should have uncertainty over $\param$ given $\param_i$ which would affect my strategy nonlinearly.}
